# Supplementary material for: CODIT: Code Editing with Tree-Based Neural Models
Source: arXiv:1810.00314 source file (2020-08-25)
Supplement: Supplementary file 1 [file appendix.tex]

\appendices
\section{Correct Patches Generated By \tool}
\begin{table*}[!htb]
    \centering
    \begin{tabular}{l}
         \toprule
Chart - 1\\
\begin{lstlisting}
- if (dataset != null)
+ if (dataset == null) 
\end{lstlisting}\\
\midrule
Chart - 9\\
\begin{lstlisting}
- if (endIndex < 0) {
+ if ((endIndex < 0)  || (endIndex < startIndex)) {  
\end{lstlisting}\\
\midrule
Chart - 11\\
\begin{lstlisting}
- PathIterator iterator2 = p1.getPathIterator(null);
+ PathIterator iterator2 = p2.getPathIterator(null); 
\end{lstlisting}\\
\midrule

Closure - 65\\
\begin{lstlisting}
-  case '\0': sb.append("\\0"); break;
+  case '\0': sb.append("\\000"); break; 
\end{lstlisting}\\
\midrule
Closure - 73\\
\begin{lstlisting}
- if (c > 0x1f && c <= 0x7f) {
+ if (c > 0x1f && c < 0x7f) { 
\end{lstlisting}\\
\midrule
Closure - 86\\
\begin{lstlisting}
- return true;
+ return false; 
\end{lstlisting}\\
\midrule
Closure - 92\\
\begin{lstlisting}
- int indexOfDot = namespace.indexOf('.');
+ int indexOfDot = namespace.lastIndexOf('.'); 
\end{lstlisting}\\
\midrule
Closure - 93\\
\begin{lstlisting}
- int indexOfDot = namespace.indexOf('.');
+ int indexOfDot = namespace.lastIndexOf('.');
\end{lstlisting}\\
\midrule
Closure - 104\\
\begin{lstlisting}
- if (result != null) {
+ if (!result.isNoType()) { 
\end{lstlisting}\\
\midrule
\midrule
Lang - 16\\
\begin{lstlisting}
- if (str.startsWith("0x") || str.startsWith("-0x")) {
+ if (str.startsWith("0x") || str.startsWith("-0x") || str.startsWith("0X") || str.startsWith("-0X")) { 
\end{lstlisting}\\
\midrule
Lang - 24\\
\begin{lstlisting}
- return foundDigit && !hasExp;
+ return foundDigit && !hasExp && !hasDecPoint; 
\end{lstlisting}\\
\midrule
Lang - 59\\
\begin{lstlisting}
- str.getChars(0, strLen, buffer, size);
+ str.getChars(0, width, buffer, size); 
\end{lstlisting}\\
\midrule
\midrule
Math - 5\\
\begin{lstlisting}
- return NaN;
+ return INF; 
\end{lstlisting}\\
\midrule
Math - 33\\
\begin{lstlisting}
- if (Precision.compareTo(entry, 0d, maxUlps) > 0) {
+ if (Precision.compareTo(entry, 0d, epsilon) > 0) {  
\end{lstlisting}\\
\midrule
Math - 57\\
\begin{lstlisting}
- int sum = 0;
+ double sum = 0; 
\end{lstlisting}\\
\midrule
Math - 70\\
\begin{lstlisting}
- return solve(min, max);
+ return solve(f, min, max); 
\end{lstlisting}\\
\midrule
Math - 75\\
\begin{lstlisting}
- return getCumPct((Comparable<?>) v);
+ return getPct((Comparable<?>) v); 
\end{lstlisting}\\
\midrule
Math - 82\\
\begin{lstlisting}
- if (MathUtils.compareTo(entry, 0, epsilon) >= 0) {
+ if (MathUtils.compareTo(entry, 0, epsilon) > 0) { 
\end{lstlisting}\\
\midrule
Math - 85\\
\begin{lstlisting}
- if (fa * fb >= 0.0 ) {
+ if (fb * fa > 0.0 ) {  
\end{lstlisting}\\
\midrule
Time - 3\\
\begin{lstlisting}
- } else if (offsetLocal > 0) {
+ } else if (offsetLocal >= 0) { 
\end{lstlisting}\\
    \end{tabular}
    \caption{Correct patches that \tool can generate successfully.}
    \label{tab:my_label}
\end{table*}
